# Supplementary material for: Evolution of noisy learning in games
Source: arXiv:2506.21498 ancillary file (2026-03-25)
Supplement: Supplementary file 1 [file supporting-information.pdf]

# Supporting Information:
# Evolution of boundedly rational learning in games

Marta C. Couto[a,b,1], Fernando P. Santos[a], and Christian Hilbe[b,c]

[a]Informatics Institute, University of Amsterdam, Amsterdam 1098XH, The Netherlands
[b]Max Planck Research Group on the Dynamics of Social Behavior, Max Planck Institute for Evolutionary Biology, 24306 Plön, Germany
[c]Interdisciplinary Transformation University IT:U, 4040 Linz, Austria
[1]To whom correspondence should be addressed. E-mail: mccouto@evolbio.mpg.de, m.gomesdacunhacouto@uva.nl

June 26, 2025

## Contents

**1 Supporting information on the model** **2**
1.1 Introspection dynamics and average payoffs . . . . . 2
1.2 Adaptive dynamics . . . . . 3
1.2.1 Evolutionary stability . . . . . 4
1.2.2 Ecological equilibrium and polymorphic populations . . . . . 4
1.2.3 Canonical equation of adaptive dynamics . . . . . 5

**2 Additional results** **6**
2.1 Super-game for a wide range of 2×2 stage games . . . . . 6
2.2 Trait evolution plots and canonical equation . . . . . 6
2.3 Stationary distribution of introspection dynamics with asymmetric selection strengths . . . . 7
2.4 Evolution of average cooperation and payoffs . . . . . 7
2.5 Evolutionary outcomes for a wider range of games . . . . . 7
2.6 Multiplayer games . . . . . 8

The present document consists of two main sections: supporting information on the model (Section 1) and additional results (Section 2). Regarding the model, here we provide all the details necessary to the theoretical analysis presented in the main text. Namely, in Section 11.1 we describe how to obtain the stationary distributions refering to the short-run dynamics. In turn, Section 11.2 is dedicated to the long-run dynamics. There, we introduce some basic concepts of adaptive dynamics that we use in our analysis. As for the additional results, they range from helping to understand the results shown in the main text to further explorations such as after-branching dynamics and multiplayer games.

# 1 Supporting information on the model

## 1.1 Introspection dynamics and average payoffs

In the main text, we provide the stationary distribution over the game outcomes when players learn through introspection dynamics and have the same selection strength, $\beta_1 = \beta_2 = \beta$ (see Equation 4 in the main text). Here, we explain how to derive that expression and also that for the case where $\beta_1 \neq \beta_2$.

We use introspection dynamics to model the short-run dynamics. Following the methods in Couto et al. [1], we represent the learning dynamics as a Markov chain whose states correspond to the four possible outcomes of the game – **CC**, **CD**, **DC**, and **DD** – defined by

$$\begin{array}{c|cc} & \mathbf{C} & \mathbf{D} \\ \hline \mathbf{C} & 1 & -B \\ \mathbf{D} & 1-A & 0 \end{array}\,. \tag{1}$$

We denote the probability that the state $i$ changes to $j$ in one time step by $T_{ij}$ (where $i, j \in \{\mathbf{CC}, \mathbf{CD}, \mathbf{DC}, \mathbf{DD}\}$). We write that transition probability using Equation 3 in Ref.[1] for a 2-strategy game where payoffs are symmetric and where the two players have different selection strengths $\beta_1 \neq \beta_2$. The transition matrix $T := (T_{ij})$ is then given by[1]

$$\begin{pmatrix} 1-\frac{1}{2(1+e^{\beta_1 A})}-\frac{1}{2(1+e^{\beta_2 A})} & \frac{1}{2(1+e^{\beta_2 A})} & \frac{1}{2(1+e^{\beta_1 A})} & 0 \\ \frac{1}{2(1+e^{-\beta_2 A})} & 1-\frac{1}{2(1+e^{-\beta_2 A})}-\frac{1}{2(1+e^{-\beta_1 B})} & 0 & \frac{1}{2(1+e^{-\beta_1 B})} \\ \frac{1}{2(1+e^{-\beta_1 A})} & 0 & 1-\frac{1}{2(1+e^{-\beta_1 A})}-\frac{1}{2(1+e^{-\beta_2 B})} & \frac{1}{2(1+e^{-\beta_2 B})} \\ 0 & \frac{1}{2(1+e^{\beta_1 B})} & \frac{1}{2(1+e^{\beta_2 B})} & 1-\frac{1}{2(1+e^{\beta_1 B})}-\frac{1}{2(1+e^{\beta_2 B})} \end{pmatrix}. \tag{2}$$

We can now obtain the stationary distribution over the game outcomes $\mathbf{u}(A, B, \beta_1, \beta_2)$ by solving the eigenvector problem

$$\begin{aligned} \mathbf{u} &= \mathbf{u}T \\ \mathbf{u}\,\mathbf{e}^\top &= 1. \end{aligned} \tag{3}$$

Here, $\mathbf{e}$ denotes the 4-dimensional row-vector where each entry is equal to 1 and the superscript $\top$ indicates transposition. Hence, the second equation is the usual normalization for a probability vector (requiring that the sum of all entries $\mathbf{u}$ is equal to 1).

For 2-strategy games, we can obtain simple analytical expressions of the stationary distribution. For the

[1] Note that the transition matrix 2 corresponds to that in page 6 of Ref.[1] for the transformations $\beta A \to \beta_1 A$, $\beta A' \to \beta_2 A$, $\beta B \to \beta_1 B$, and $\beta B' \to \beta_2 B$. This is so because the learning dynamics of our game is equivalent to that of an asymmetric game in which (otherwise symmetric) payoffs are scaled by each player's respective selection strengths.

case $\beta_1 = \beta_2 = \beta$, that is

$$\mathbf{u}(A,B,\beta,\beta) = \frac{1}{2+e^{A\beta}+e^{B\beta}}(e^{A\beta},1,1,e^{B\beta}), \tag{4}$$

as provided in the main text. Here, we also show the more complex expression for the asymmetric case $\beta_1 \neq \beta_2$,

$$\begin{aligned}\mathbf{u}(A,B,\beta_1,\beta_2) = \frac{1}{f}(&e^{(A+B)\beta_1} + e^{(A+B)\beta_2} + 2e^{A(\beta_1+\beta_2)} + 2e^{A(\beta_1+\beta_2)+B\beta_1} + 2e^{A(\beta_1+\beta_2)+B\beta_2},\\ &2e^{A\beta_1} + 2e^{B\beta_2} + e^{(A+B)\beta_1} + e^{(A+B)\beta_2} + 2e^{A\beta_1+B\beta_2},\\ &2e^{B\beta_1} + 2e^{A\beta_2} + e^{(A+B)\beta_1} + e^{(A+B)\beta_2} + 2e^{A\beta_2+B\beta_1},\\ &e^{(A+B)\beta_1} + e^{(A+B)\beta_2} + 2e^{B(\beta_1+\beta_2)} + 2e^{A\beta_1+B(\beta_1+\beta_2)} + 2e^{A\beta_2+B(\beta_1+\beta_2)}),\end{aligned} \tag{5}$$

where $f$ is a normalization factor given by

$$\begin{aligned}f = 2\Big(&e^{A\beta_1} + e^{A\beta_2} + e^{B\beta_1} + e^{B\beta_2} + e^{A(\beta_1+\beta_2)} + e^{B(\beta_1+\beta_2)} + 2e^{(A+B)\beta_1} + 2e^{(A+B)\beta_2} + \\ &+ e^{A\beta_1+B\beta_2} + e^{A\beta_2+B\beta_1} + e^{A\beta_1+B(\beta_1+\beta_2)} + e^{A\beta_2+B(\beta_1+\beta_2)} + e^{A(\beta_1+\beta_2)+B\beta_1} + e^{A(\beta_1+\beta_2)+B\beta_2}\Big).\end{aligned} \tag{6}$$

Finally, we can also write the average payoff of a player with $\beta = \beta_1$ against a player with $\beta = \beta_2$ as

$$\Pi_{\beta_2}(\beta_1) = \mathbf{u}(A,B,\beta_1,\beta_2)\cdot(1,-B,1-A,0), \tag{7}$$

which yields

$$\begin{aligned}\Pi_{\beta_2}(\beta_1) =& \frac{1}{f}\left(-2B(e^{A\beta_1} + e^{B\beta_2} + e^{A\beta_1+B\beta_2}) + 2(1-A)(e^{A\beta_2} + e^{B\beta_1} + e^{A\beta_2+B\beta_1})\right.\\ &\left.+ 2(e^{A(\beta_2+\beta_1)} + e^{A(\beta_2+\beta_1)+B\beta_2} + e^{A(\beta_2+\beta_1)+B\beta_1}) - (A+B-2)(e^{(A+B)\beta_1} + e^{(A+B)\beta_2})\right).\end{aligned} \tag{8}$$

This equation is crucial for most of our results. Ultimately, it allows us to numerically produce Figure 4 of the main text.

## 1.2 Adaptive dynamics

In this section, we introduce some basic concepts of adaptive dynamics that we use in our subsequent analysis for the evolution of selection strengths. In the main text, we already define the key concepts of *invasion fitness*, *local fitness gradient* (or *selection gradient*), and *singular point* and respective evolutionary stability properties. Here, we extend some of these notions and introduce the *canonical equation* of adaptive dynamics. For that we follow Refs.[2–5].

In the following, we often need to refer to the selection strength of the resident population, and to the selection strength of a mutant. To distinguish those two variables, it is convenient to use $x$ or $x_i$ ($i = 1, 2, \dots$) to refer to the resident's selection strength trait or traits, and $y$ to refer to the mutant's trait.

### 1.2.1 Evolutionary stability

We recall the definition given in the main text of the invasion fitness of a mutant with $\beta = y$ in a monomorphic resident population $\beta = x$,

$$s_x(y) := \Pi_x(y) - \Pi_x(x), \tag{9}$$

where $\Pi_x(y)$ is given by Equation 8. This is a central quantity as its properties are informative of the system's evolutionary fate. If $s_x(y)$ is positive, a mutant with trait $y$ can invade a resident population with trait $x$. If $s_x(y)$ is negative, the respective mutant is expected to go extinct.

The selection gradient is the derivative of the invasion fitness evaluated at the resident population $x$,

$$D(x) := \left[\frac{\partial s_x(y)}{\partial y}\right]_{y=x}. \tag{10}$$

Thus, the selection gradient determines the direction of evolutionary change. When $D(x)$ is positive (negative), mutants with a slightly higher (lower) trait value than $x$ can replace the resident population. Therefore, we would expect the population's trait value to increase (decrease).

A point $x^*$ that satisfies $D(x^*) = 0$ is called evolutionary singular. Evolutionary singular points can have several properties regarding their stability. Let us define

$$\begin{aligned} a := a(x^*) &:= \left[\frac{\partial^2 s_x(y)}{\partial x^2}\right]_{y=x=x^*} \\ b := b(x^*) &:= \left[\frac{\partial^2 s_x(y)}{\partial y^2}\right]_{y=x=x^*}. \end{aligned} \tag{11}$$

We characterize the singular point as follows [2].

i If $b < 0$, no nearby mutant can invade; therefore, the singular point is *evolutionarily stable*;

ii If $a - b < 0$, a population of a nearby trait can be invaded by mutants that are closer to $x^*$; therefore, the singular point is *convergence-stable*;

iii If $a > 0$, the singular trait $x^*$ can invade populations of a slightly different trait when initially rare itself;

iv If $a + b < 0$, all pairs of traits near the singular point can mutually invade each other; therefore, there are nearby dimorphisms.

If (i) and (ii) are satisfied, $x^*$ is called *continuously stable.* This means that the singular trait corresponds to an evolutionary endpoint. If (ii) is satisfied but not (i), $x^*$ is an *evolutionary branching point.*

### 1.2.2 Ecological equilibrium and polymorphic populations

While adaptive dynamics often describes transitions from one homogeneous population to another, the system can also reach a point where the mutant does not completely replace the resident population. This occurs when the resident and mutant traits can mutually invade (for example, at a branching point), creating a dimorphism where the two traits coexist. In the following, we describe how to deal with those cases.

By the common assumption that mutations are rare, a resident population reaches an *ecological equilibrium* before a new mutant appears. Usually, that means a mutant either dies out or fixates in the population before a new one is introduced. However, if coexistence is allowed, there will be a stable ecological equilibrium among the different types present in the population. The ecological equilibrium can also be regarded as

the replicator equation equilibrium [5]. Hence, at equilibrium, all individuals have the same fitness (average payoff). If there are two coexisting types $x_1$ and $x_2$, we can calculate the ecological equilibrium point $p$, denoting the proportion of type $x_1$ in the population, by solving

$$p\,\Pi_{x_1}(x_1) + (1-p)\,\Pi_{x_2}(x_1) = p\,\Pi_{x_1}(x_2) + (1-p)\,\Pi_{x_2}(x_2), \tag{12}$$

where the left-hand side refers to the average payoff of type $x_1$ and the right-hand side refers to the average payoff of type $x_2$, assuming a well-mixed population. The ecological stability is guaranteed because, by definition, the two present types must be able to mutually invade. Moreover, the uniqueness of the stable equilibrium point is guaranteed by the average payoffs being linear on the types' frequency $p$.

Similarly, when there are three types, $x_1$, $x_2$ and $x_3$, we obtain the equilibrium point $(p_1, p_2)$, where $p_1$ and $p_2$ respectively denote the proportion of types $x_1$ and $x_2$, by solving

$$\begin{aligned} p_1\,\Pi_{x_1}(x_1) + p_2\,\Pi_{x_2}(x_1) + (1-p_1-p_2)\,\Pi_{x_3}(x_1) &= p_1\,\Pi_{x_1}(x_2) + p_2\,\Pi_{x_2}(x_2) + (1-p_1-p_2)\,\Pi_{x_3}(x_2) \\ p_1\,\Pi_{x_1}(x_1) + p_2\,\Pi_{x_2}(x_1) + (1-p_1-p_2)\,\Pi_{x_3}(x_1) &= p_1\,\Pi_{x_1}(x_3) + p_2\,\Pi_{x_2}(x_3) + (1-p_1-p_2)\,\Pi_{x_3}(x_3). \end{aligned} \tag{13}$$

We can thereby generalize the concept of invasion fitness to a polymorphic system. Suppose there are $n$ different types or traits. Let the invasion fitness of a mutant $y$ in a resident population with traits $x_1, x_2, \ldots, x_n$ at its ecological equilibrium be $s_{x_1,x_2,\ldots,x_n}(y)$. We define the direction of evolution of the $x_i$-trait by

$$D_i(x_1, x_2, \ldots, x_n) := \left[\frac{\partial s_{x_1,x_2,\ldots,x_n}(y)}{\partial y}\right]_{y=x_i}. \tag{14}$$

For example, for $n = 2$, we get

$$D_i(x_1, x_2) := \left[\frac{\partial s_{x_1,x_2}(y)}{\partial y}\right]_{y=x_i}, \tag{15}$$

for $i = 1, 2$, where

$$s_{x_1,x_2}(y) = \Pi_{x_1,x_2}(y) - \Pi_{x_1,x_2}(x_1), \tag{16}$$

where

$$\begin{aligned} \Pi_{x_1,x_2}(y) &= p\,\Pi_{x_1}(y) + (1-p)\,\Pi_{x_2}(y) \\ \Pi_{x_1,x_2}(x_1) &= p\,\Pi_{x_1}(x_1) + (1-p)\,\Pi_{x_2}(x_1). \end{aligned} \tag{17}$$

Remind that at ecological equilibrium $p$, $\Pi_{x_1,x_2}(x_1) = \Pi_{x_1,x_2}(x_2)$.

### 1.2.3 Canonical equation of adaptive dynamics

Since the selection gradients give the direction of trait evolution, we can use them to write differential equations describing a deterministic approximation of the evolutionary dynamics. Such equations are called the *canonical equations* of adaptive dynamics [4]. For $n = 1$, it can take the form of

$$\dot{x} = C_0\, D(x). \tag{18}$$

For $n = 2$,

$$\begin{aligned} \dot{x_1} &= C_1\, p\, D_1(x_1, x_2), \\ \dot{x_2} &= C_2\,(1-p)\, D_2(x_1, x_2). \end{aligned} \tag{19}$$

Finally, for $n = 3$,

$$\begin{aligned}\dot{x_1} &= C_1\, p_1\, D_1(x_1, x_2, x_3),\\ \dot{x_2} &= C_2\, p_2\, D_2(x_1, x_2, x_3),\\ \dot{x_3} &= C_3\,(1 - p_1 - p_2)\, D_3(x_1, x_2, x_3).\end{aligned} \tag{20}$$

$C_0$, $C_1$, $C_2$ and $C_3$ are constant coefficients [3, 4].

We use the concept of mutual invasibility and the canonical equations in **Fig. S2**, where we explore the dynamics of a stag-hunt game after evolutionary branching has occurred. We provide further details in the respective section.

# 2 Additional results

## 2.1 Super-game for a wide range of 2×2 stage games

We refer to the interaction among players with different selection strengths as a *super-game*. Specifically, in a super-game, strategies are defined by a player's selection strength and the respective payoffs result from the introspection dynamics stationary distribution (see **Fig. 2D, H** of the main text). In **Fig. 2D**, the high $\beta$ dominates the low $\beta$ (in this case, $\beta = 5$ dominates $\beta = 2$). As for the example in **Fig. 2H**, it is the low selection strength that dominates. Each of these two examples correspond to one particular stage game and one pair of selection strength values. We can do the same exercise for any 2×2 stage game, and any values of $\beta$. In **Fig. S1**, we show the resulting super-game for three different pairs of selection strengths and a wide range of stage games. Besides dominance, we also find many super-games that take the form of an anti-coordination game. There, players prefer to have the opposite selection strength than their opponent. In addition, we also find a few coordination games, where a player prefers to have a high $\beta$ only if the co-player has a high $\beta$ too.

## 2.2 Trait evolution plots and canonical equation

In the main text, we have seen that stag-hunt games can lead to evolutionary branching; here, we would like to further explore the subsequent dynamics, after branching has occurred. In **Fig. S2**, we show in more detail the branching case presented in the main text. First, we show the pairwise invasibility plot (**Fig. S2A**), same as in **Fig. 3F** of the main text, where we can see the singular branching point. Then, a *trait evolution plot* [2, 4] (**Fig. S2B**) highlights which trait types can coexist. The gray shaded area corresponds to trait pairs $x_1$ and $x_2$ that can mutually invade, that is, $s_{x_1}(x_2) > 0$ and $s_{x_2}(x_1) > 0$. Therefore, we can obtain a trait evolution plot by overlapping the original pairwise invasibility plot with its mirror image (obtained by inverting the pairwise invasibility plot with respect to the main diagonal.) We can focus on the half above the diagonal only, defining the low trait (branch) to be $x_1$ and the high trait to be $x_2$. The lower half of the plot corresponds to the symmetric case. The gradient $(D_1(x_1, x_2), D_2(x_1, x_2))$ (gray vector field overlapping the shaded area) shows the direction of evolution of branches $x_1$ and $x_2$; the colored lines correspond to isoclines (where $D_1$ or $D_2$ vanish). In this case, the isoclines do not intersect – there is always change at least in one of the directions. In particular, the upper branch $x_2$ keeps growing (the gradient points upwards), while the bottom branch $x_1$ seems to stabilize somewhere between 1 and 2. We confirm that by solving the canonical equation numerically (**Fig. S2C**). This analysis also reveals that the subpopulation corresponding to the lower branch is quite larger, reaching an abundance of about 79% (**Fig. S2C**, bottom).

## 2.3 Stationary distribution of introspection dynamics with asymmetric selection strengths

Here, we show an analogous figure to **Fig. 2** in the main text for two other games, the stag-hunt game (**Fig. S3A**–**D**) and the weak prisoner's dilemma, that is, for small $|A|$ (**Fig. S3E**–**H**).

In the stag-hunt game, as we increase the rationality $\beta$ of both players (**Fig. S3A**–**B**), players increasingly learn to play **D** – because that is the risk-dominant strategy. Therefore, when both players adopt the more effective learning strategy (**Fig. S3B**), both of them get a low payoff close to zero. In this scenario, we observe that the super-game takes the form of an anti-coordination game (**Fig. S3D**). That is, when both players are highly effective learners, there is an incentive to deviate to the less effective learning strategy. The less effective learner would then play **C** for a substantial amount of time. The more effective learner would then best-respond, which in turn makes them play **C** a considerable amount of time, too. This translates into higher payoffs for both players, providing an intuition for why branching occurs.

For a weak prisoner's dilemma in which the absolute value $|A|$ is small, the gain in deviating from mutual cooperation is small compared to the mutual cooperation reward. Therefore, by increasing one's $\beta$ (player 1 in **Fig. S3E to G**), the small gain from increasing state **DC** is not enough to compensate for the increase in mutual defection (at the cost of decreasing mutual cooperation). Here, it therefore does not pay to increase one's learning effectiveness. At the same time, lowering one's $\beta$ (player 2 in **Fig. S3F to G**), and hence cooperating more, induces the co-player to cooperate slightly more, too, since there is less risk of being the sucker. That yields an increase in both players' average payoff. This shows that even in a prisoner's dilemma, the strictest kind of social dilemma, we can see the emergence of bounded rationality.

## 2.4 Evolution of average cooperation and payoffs

In **Fig. S4** we show how the players' average cooperation rates and their average payoffs change according to the long-run dynamics, along with the trait $\beta$. For that, we assume all individuals in the population interact with each other. From time to time during a simulation, we then calculate the average cooperation rate and the payoff of an individual against every other. The average payoff is computed using (7). The average cooperation by a player with $\beta_1$ in an interaction with a player with $\beta_2$ is given by $u_{\mathbf{CC}}(A, B, \beta_1, \beta_2) + u_{\mathbf{CD}}(A, B, \beta_1, \beta_2)$. We then take the mean over all individuals in the population. Individuals start by cooperating half of the time since the initial population has $\beta = 0$. With increasing $\beta$, cooperation drops. Only in the stag-hunt game there is an increase in cooperation, after the branching point (**Fig. S4C**).

## 2.5 Evolutionary outcomes for a wider range of games

In **Fig. S5**, we extend the range of one-shot games considered in **Fig. 4** of the main text. We obtain the same overall dynamics, except in the quadrant corresponding to stage games of the snowdrift type. In this quadrant, there is a white strip close to the diagonal for which there is no singular strategy. In the main text, we explained why for a particular snowdrift game we observe the evolution towards a finite value of $\beta$. The general mechanism for that to happen is the following. When players with different $\beta$ meet, the one with lower $\beta$ is more prone to mistakes, that is, to deviate from one of the two Nash equilibria. Also, they will more likely deviate from a Nash equilibria when it is less costly to do so. The player with higher $\beta$ will respond quicker to an unfavorable state by playing their best-response. If, at the same time, this response makes them being in the less preferred outcome, then a player has no incentive to have the higher $\beta$. Therefore, the conditions for the evolution of a finite value of $\beta$ are:

1. **CD** is less preferred than **DC** to the row-player *and* deviations from **DC** are less costly to the column-player than deviations from **CD** *or*

2. **DC** is less preferred than **CD** to the row-player *and* deviations from **CD** are less costly to the column-player than deviations from **DC**.

This translates into

$$\Big(-B < 1-A \ \wedge \ 0-(-B) > 1-(1-A)\Big) \vee \Big(-B > 1-A \ \wedge \ 0-(-B) < 1-(1-A)\Big). \tag{21}$$

These conditions can be simplified to

$$\big(B > A\big) \ \vee \ \big(B < A-1\big). \tag{22}$$

The expression in the first bracket refers to the top triangle in the snowdrift quadrant. The expression in the second bracket refers to the bottom triangle.

## 2.6 Multiplayer games

In the main text, we have focussed on simple matrix games among two players only. In the following, we briefly consider some special cases of multiplayer games. In particular, we analyze linear, discounted and threshold public goods games. These games are considered multiplayer versions of the prisoner's dilemma, snowdrift and stag-hunt games, respectively.

Again, we assume two strategies only. Players can either cooperate (**C**) by contributing to a common pool, or they defect (**D**) and contribute nothing. In the linear public goods game, each player decides whether to contribute or not a benefit $r$ to the common pool at a cost of $c$. The sum of all contributions is equally divided among all $N$ players. Thus, if a group has $k$ cooperators, the payoffs of defectors and cooperators are, respectively,

$$\begin{aligned} \pi^{\mathbf{D}}(k) &= \frac{r}{N}k, \\ \pi^{\mathbf{C}}(k) &= \pi^{\mathbf{D}}(k) - c. \end{aligned} \tag{23}$$

The discounted public goods game is similar to the linear public goods game. However, here each additional contribution to the common pool gets discounted by a factor of $w < 1$, see Ref. [6]. The payoffs are

$$\begin{aligned} \pi^{\mathbf{D}}(k) &= \frac{r}{N}(1 + w + w^2 + ... + w^{k-1}), \\ \pi^{\mathbf{C}}(k) &= \pi^{\mathbf{D}}(k) - c. \end{aligned} \tag{24}$$

In the threshold public goods game, the sum of contributions are only redistributed among all players if a certain number of cooperators $M$ is reached [7, 8]. The payoffs are defined as

$$\begin{aligned} \pi^{\mathbf{D}}(k) &= \frac{r}{N}\Theta(k - M), \\ \pi^{\mathbf{C}}(k) &= \pi^{\mathbf{D}}(k) - c. \end{aligned} \tag{25}$$

Here, $\Theta(x)$ is the Heaviside function defined by $\Theta(x) = 1$ if $x \geq 0$ and $\Theta(x) = 0$ otherwise.

The expressions for the stationary distribution of introspection dynamics of multiplayer games [9] becomes much more cumbersome. As a result, an exact computation of singular points of the respective adaptive dynamics is no longer possible. We show, however, the pairwise invasibility plots for 3-player games

in **Fig. S6**. We find that the qualitative evolutionary outcomes are consistent with the respective 2-player game types in the main text.

# References


[1] MC Couto, S Giaimo, C Hilbe, Introspection dynamics: A simple model of counterfactual learning in asymmetric games. *New Journal of Physics* **24**, 63010 (2022).

[2] SAH Geritz, E Kisdi, G Meszéna, JAJ Metz, Evolutionarily singular strategies and the adaptive growth and branching of the evolutionary tree. *Evolutionary Ecology Research* **12**, 35–57 (1998).

[3] U Dieckmann, R Law, The dynamical theory of coevolution: a derivation from stochastic ecological processes. *Journal of Mathematical Biology* **34**, 579–612 (1996).

[4] Å Brännström, J Johansson, N von Festenberg, The Hitchhiker's guide to adaptive dynamics. *Games* **4**, 304–328 (2013).

[5] M Doebeli, C Hauert, T Killingback, The evolutionary origin of cooperators and defectors. *Science* **306**, 859–62 (2004).

[6] C Hauert, F Michor, MA Nowak, M Doebeli, Synergy and discounting of cooperation in social dilemmas. *Journal of Theoretical Biology* **239**, 195–202 (2006).

[7] M Archetti, I Scheuring, Review: Evolution of cooperation in one-shot social dilemmas without assortment. *Journal of Theoretical Biology* **299**, 9–20 (2012).

[8] JM Pacheco, FC Santos, MO Souza, B Skyrms, Evolutionary dynamics of collective action in n-person stag hunt dilemmas. *Proceedings of the Royal Society B* **276**, 315–321 (2009).

[9] MC Couto, S Pal, Introspection Dynamics in Asymmetric Multiplayer Games. *Dynamic Games and Applications* (2023).

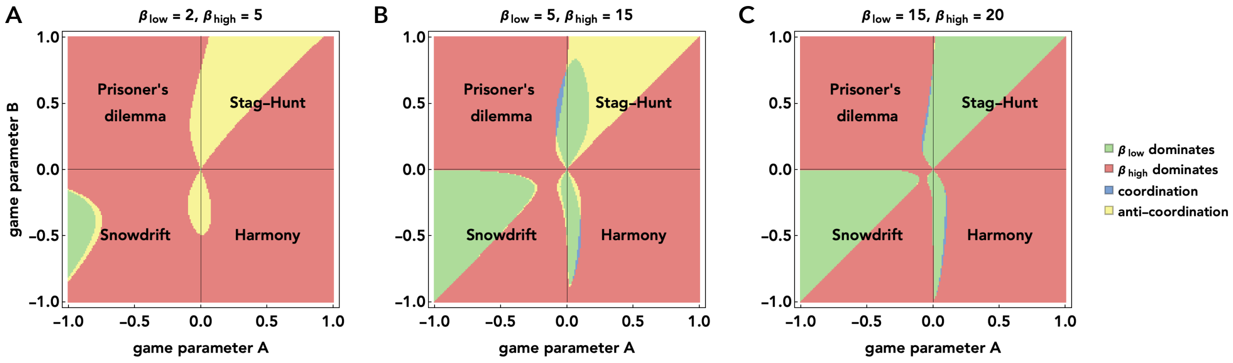


**Figure S1: Super-games for a wide range of 2×2 social dilemmas.** We fix three pairs of selection strengths: **A,** low selection strengths (2 and 5), **B,** intermediate selection strengths (5 and 15), and **C,** high selection strengths (15 and 20). Then we show, by varying the parameters $A$ and $B$, for each stage game, the type of super-game that is created – low-$\beta$ dominance, high-$\beta$ dominance, coordination or anti-coordination.

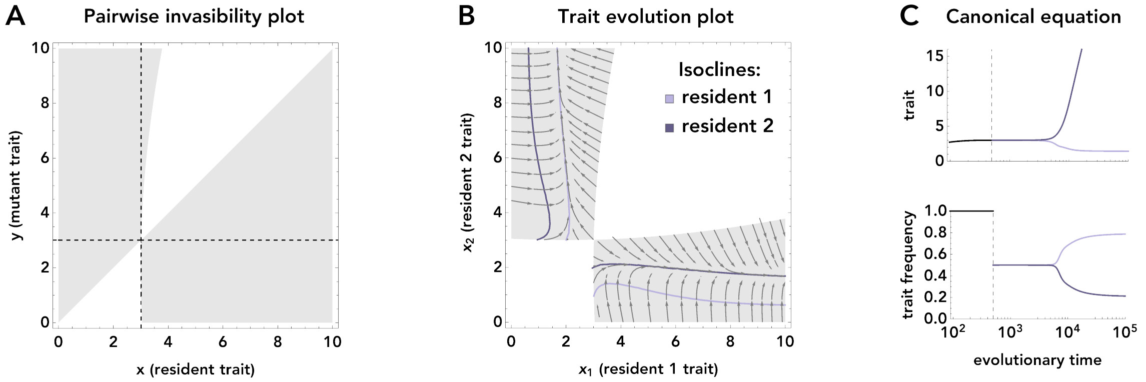


**Figure S2: Pairwise invasibility plots (A), trait evolution plots (B) and canonical equation (C) of the stag-hunt game with** $A = 0.1, B = 0.8$**. A,** Shaded area shows $s_x(y) > 0$, as before. The dashed lines correspond to the singular points. **B,** Shaded area shows $s_{x_1}(x_2) > 0$ and $s_{x_2}(x_1) > 0$. The vector field corresponds to the gradient $(D_1(x_1, x_2), D_2(x_1, x_2))$, showing the direction of evolution. The colored lines correspond to isoclines, where $D_1$ or $D_2$ vanish, respectively. **C,** Canonical equation. We solve the canonical equations 18 and 19 numerically. The dashed line marks the branching point. The initial trait is 0, and $C_0 = 2$, $C_1 = C_2 = 5$. The trait frequencies are obtained by solving the ecological equilibrium condition Eq. 12.

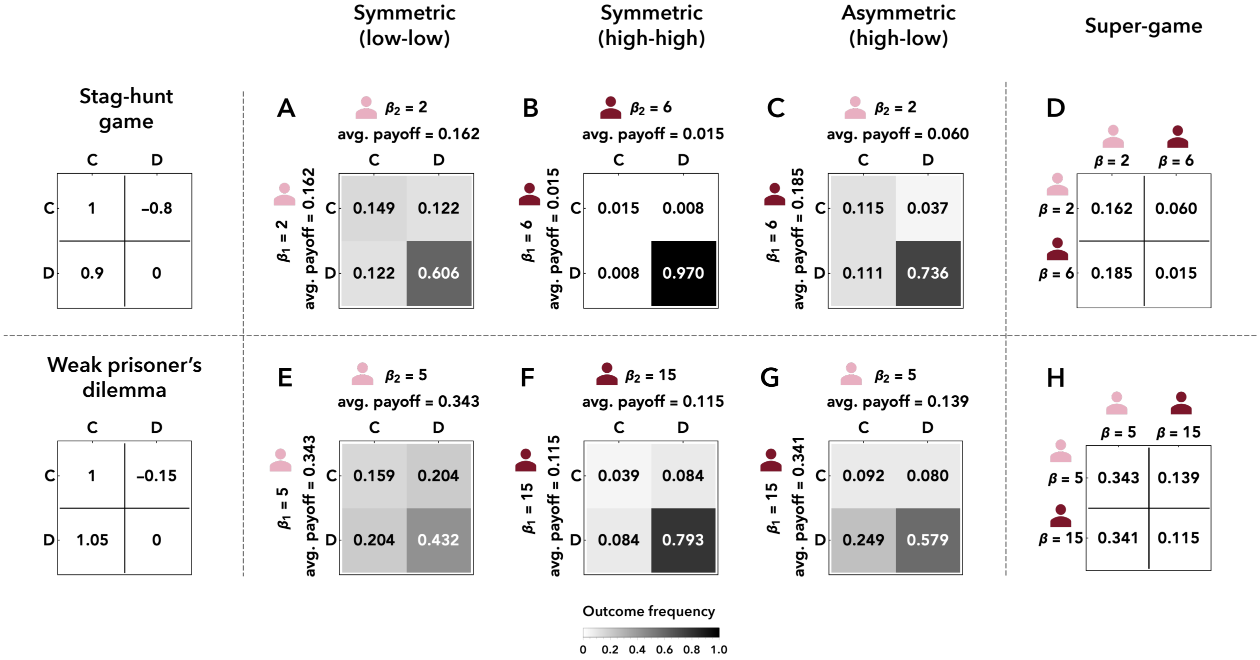


**Figure S3: Introspection dynamics among players with different selection strengths**. **A–D,** Stag-hunt game ($A = 0.1, B = 0.8$). **E–H,** Weak prisoner's dilemma ($A = -0.05, B = 0.15$). The stationary distribution is depicted by the black and white gradient – the darker the shading, the more frequent the game outcome. The numerical values of the stationary distribution are also shown. The average payoffs are calculated using Eq. 7.

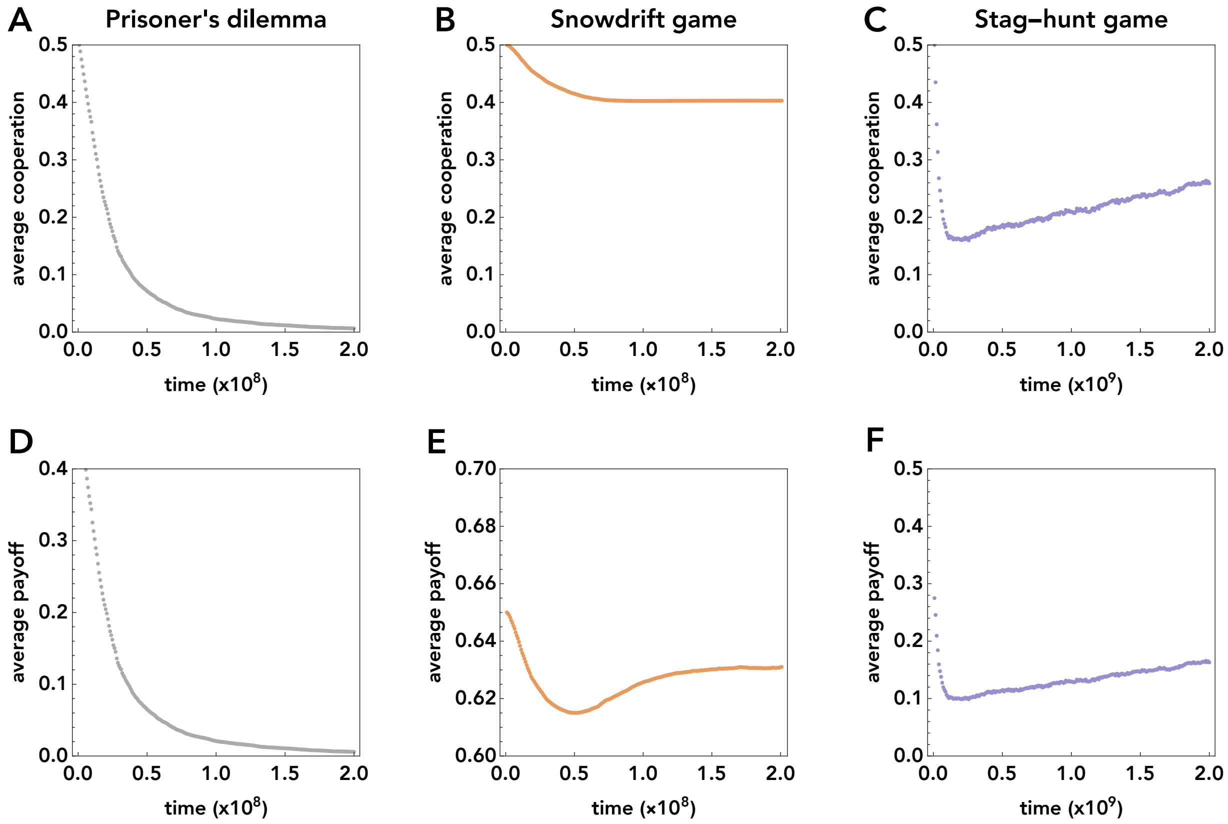


**Figure S4: Average cooperation (A–C) and average payoffs (D–E) over evolutionary time.** These are results from the same simulations shown in **Fig. 3** in the main text.

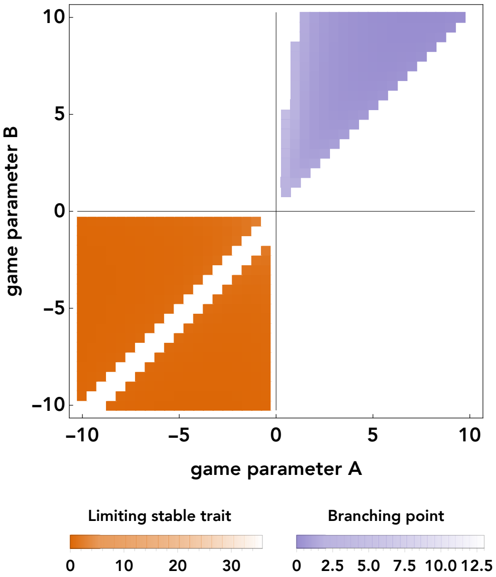


**Figure S5: Evolutionary outcomes across 2-strategy social dilemmas.** We solve the equation $D(x^*) = 0$ for games in the shown range. When there is a solution $x^*$ (colored), we derive its stability properties. In orange, the games that lead to a convergent and evolutionary stable trait. In purple, the games that lead to a convergent but unstable point, that is, a branching point. The color gradient represents the singular trait: the lighter, the higher the trait value is. When there is no solution to $D(x^*) = 0$, we verify that $D(x)$ is always positive (white). The game parameters $A$ and $B$ range between $-10$ and 10, in a 0.5 step.

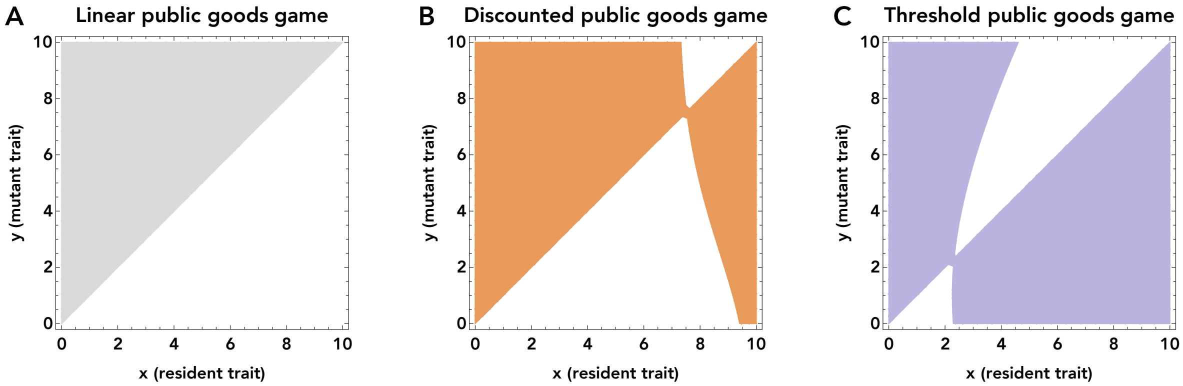


**Figure S6: Pairwise invasibility plots for multiplayer games.** As before, the shaded areas represent a positive invasion fitness. **A,** Linear public goods game. The payoffs are defined by Eq. 23 with $N = 3$, $r = 2$, $c = 0.2$. **B,** Discounted public goods game. The payoffs are defined by Eq. 24 with $N = 3$, $r = 2$, $c = 0.2$, and $w = 0.5$. **C,** Threshold public goods game. The payoffs are defined by Eq. 25 with $N = 3$, $r = 2$, $c = 1$, and $M = 2$.
